# Supplementary material for: GypSum: Learning Hybrid Representations for Code Summarization
Source: arXiv:2204.12916 source file (2022-04-26)
Supplement: Supplementary file 1 [file appendix.tex]

\appendix
\setcounter{table}{0}
\setcounter{figure}{0}
\section{Appendix}

\subsection{Additional Case Study}
We present more example summaries generated by different models in this section. Table~\ref{tab:append_java} and Table~\ref{tab:append_python} show the examples for Java and Python code, respectively. Our GypSum model can generate fluent and informative summaries, which are the closest to the ground-truth text.

\begin{table*}[!t]
\small
\centering
  \caption{The summary examples generated by different models for Java code.}
    \label{tab:append_java}
      \begin{tabular}{p{0.9\textwidth}}
      \hline
\begin{lstlisting}[style = java]
private static boolean renderFrame ( int [] pixels , long gifFileInPtr , int [] metaData )
{
    this.render(pixels,gifFileInPtr,metaData,0);
}
\end{lstlisting} \\

\textcolor{green}{Ground-Truth:}  decodes a frame if needed.\\
\textcolor{red}{GypSum:}          render a gif image frame.\\
\textcolor{blue}{CodeBert:}     render a image frame.\\
\textcolor{purple}{CodeT5:} render the frame as a gif image.\\
\textcolor{cyan}{SiT:}     render the frame as a frame.	\\
\textcolor{orange}{Transformer:}   render the frame file.\\
% \textcolor{purple}{DeepCom:}        return render a frame file.\\
\\
\hline

\begin{lstlisting}[style = java]
@Override 
public String execute ( ) 
{ 
    return SUCCESS ; 
}
\end{lstlisting} \\

\textcolor{green}{Ground-Truth:} default : just returns " success ".\\
\textcolor{red}{GypSum:}  default method - returns "success".\\
\textcolor{blue}{CodeBert:} just return "success".\\
\textcolor{purple}{CodeT5:} execute the action.\\
\textcolor{cyan}{SiT:} execute the action.\\
\textcolor{orange}{Transformer:} current operation is performed.\\
% \textcolor{purple}{DeepCom:} return string if execute success.\\
\\
\hline

\begin{lstlisting}[style = java]
public boolean containsWordBreakingChar ( final @NonNull CharSequence input ){ 
    if ( ! TextUtils . isEmpty ( input ) ) { 
        for ( int i = _NUM ; i < input . length ( ) ; i ++ ) { 
            char c = input . charAt ( I ) ; 
            if ( isWordBreakingChar ( c ) ) 
                return _BOOL ; 
        } 
    } 
    return _BOOL ;
 }
\end{lstlisting} \\

\textcolor{green}{Ground-Truth:} returns true if the input string contains a word-breaking character.\\
\textcolor{red}{GypSum:}  return true if the string contains word breakpoint characters.\\
\textcolor{blue}{CodeBert:} return true if the input charsequence contains a word.\\
\textcolor{purple}{CodeT5:} check whether the given input string contains the given character sequence.\\
\textcolor{cyan}{SiT:}  returns true if the input string contains an empty character.\\
\textcolor{orange}{Transformer:} return true if contains word breaking characters.\\
% \textcolor{purple}{DeepCom:} return true if contains break char in word.\\
\\
\hline

% \iffalse
\begin{lstlisting}[style = java]
public boolean canRead () 
{
    return _is != null ; 
}
\end{lstlisting} \\

\textcolor{green}{Ground-Truth:} returns true if the associated file is readable.\\
\textcolor{red}{GypSum:}  checks if the stream is readable.\\
\textcolor{blue}{CodeBert:} return true if can be read.\\
\textcolor{purple}{CodeT5:} checks if the underlying resource can read.\\
\textcolor{cyan}{SiT:} checks if the underlying resource can read.\\
\textcolor{orange}{Transformer:} the readability of the read object.\\
% \textcolor{purple}{DeepCom:} null if the file can be read.\\
\\
\hline
% \fi

\end{tabular}
\end{table*}

\begin{table*}[!t]
\small
\centering
  \caption{The summary examples generated by different models for Python code}
    \label{tab:append_python}
      \begin{tabular}{p{0.9\textwidth}}
      \hline
\begin{lstlisting}[style = python]
def link(src, dst):
  	 if (os.name == u'nt'):
	  	 if (ctypes.windll.kernel32.CreateHardLinkW(dst, src, 0) == 0):
	  	  	 raise ctypes.WinError()
	 else:
	  	 os.link(src, dst)
\end{lstlisting} \\

\textcolor{green}{Ground-Truth:}  create a file link from source to destination.\\
\textcolor{red}{GypSum:}          create a hard-link between source and destination.\\
\textcolor{blue}{CodeBert:}     create a file-link between source and destination.\\
\textcolor{purple}{CodeT5:}  create a link from source to destination.\\
\textcolor{cyan}{SiT:} create link from source to destination .\\
\textcolor{orange}{Transformer:}   create a soft/synt link from destination.\\
% \textcolor{purple}{DeepCom:}        create a link from source to destination.\\
\\
\hline

\begin{lstlisting}[style = python]
def _is_s3_url(url):
  	 try:
	  	 return (parse_url(url).scheme in ['s3', 's3n', 's3a'])
	 except:
	  	 return False
\end{lstlisting} \\

\textcolor{green}{Ground-Truth:} default : check for an s3 url.\\
\textcolor{red}{GypSum:}  return true if url is a s3 bucket.\\
\textcolor{blue}{CodeBert:} return true if is s3 url.\\
\textcolor{purple}{CodeT5:} whether is a s3 url.\\
\textcolor{cyan}{SiT:} return true if is valid s3 url.\\
\textcolor{orange}{Transformer:} return true if the given url is a s3:// / a.\\
% \textcolor{purple}{DeepCom:} whether is a s3 url.\\
\\
\hline

\begin{lstlisting}[style = python]
def user_agent():
  	 from requests.utils import default_user_agent
	 return (('ka-lite/%s 	 ' % VERSION) + default_user_agent())
\end{lstlisting} \\

\textcolor{green}{Ground-Truth:} http user-agent header string derived from version.\\
\textcolor{red}{GypSum:} builds a user-agent string to be used in rest requests.\\
\textcolor{blue}{CodeBert:} builds a user-agent for requests.\\
\textcolor{purple}{CodeT5:} return user agent for requests.\\
\textcolor{cyan}{SiT:} build a user-agent from header.\\
\textcolor{orange}{Transformer:} builds a name using the default user agent header.\\
% \textcolor{purple}{DeepCom:} return user agent for requests.\\
\\
\hline

\begin{lstlisting}[style = python]
def exec_query(cmd, fields):
  	 if (conf.prog.powershell is None):
	  	 return _exec_query_vbs(cmd, fields)
	 return _exec_query_ps(cmd, fields)
\end{lstlisting} \\

\textcolor{green}{Ground-Truth:} execute a system query using powershell if it is available.\\
\textcolor{red}{GypSum:}  executes a powershell query.\\
\textcolor{blue}{CodeBert:} execute a powershell command.\\
\textcolor{purple}{CodeT5:} execute a query from command.\\
\textcolor{cyan}{SiT:} executes query in powershell.\\
\textcolor{orange}{Transformer:} executes commands based on a list of fields.\\
% \textcolor{purple}{DeepCom:}  execute a query from command.\\
\\
\hline

\iffalse
\begin{lstlisting}[style = python]

def directory_exists(path):
  	 return os.path.isdir(os.path.expanduser(path))

\end{lstlisting} \\

\textcolor{green}{Ground-Truth:} tests to see if path is a valid directory.\\
\textcolor{red}{GypSum:} check to see if the dirctory already exists.\\
\textcolor{orange}{CodeBert:} check if directory exists.\\
\textcolor{purple}{CodeT5:} return true if file exists.\\
\textcolor{cyan}{SiT:}     render a image frame.\\
\textcolor{orange}{Transformer:} check if a directory exists.\\
% \textcolor{purple}{DeepCom:}  return true if file exists.\\
\\
\hline
\fi
\iffalse
\begin{lstlisting}[style = python]

def get_username_for_svn_txn(repo_path, txn_id):
    return subproc_check_output(['svnlook', 'author',\ 
           repo_path, '-t', txn_id]).strip()

\end{lstlisting} \\

\textcolor{green}{Ground-Truth:} returns username for an svn transaction.\\
\textcolor{red}{GypSum:} returns the username for an svn transaction.\\
\textcolor{blue}{CodeBert:} returns svn username and no username.\\
\textcolor{purple}{CodeT5:} return the username of a svnlook.\\
\textcolor{cyan}{SiT:} get username from svn output.\\
\textcolor{orange}{Transformer:} get username from svn output.\\
% \textcolor{purple}{DeepCom:}  return the username of a svnlook.\\
\\
\hline
\fi
\end{tabular}
\end{table*}
